# Supplementary material for: Beam Stacking Experiment at a Fixed Field Alternating Gradient Accelerator
Source: arXiv:2407.13962 source file (2024-07-19)
Supplement: Supplementary file 1 [file appendixSymbol.tex]

\textcolor{red}{
\\
$A$, bucket area\\
$D_x$, dispersion function\\
$\tilde{D_x}$, average dispersion function\\
$E_i$, total energy of individual particle\\
$E_\textrm{ref}$, total energy at reference momentum\\
$E_k$, kinetic energy\\
$E_{k0}$, nominal kinetic energy\\
$\Delta E_{k}$, deviation of kinetic energy from its nominal value\\
$E_{stack}$, target energy of stacking\\
$E_{acc,1}$, energy of beam 1\\
$E_{acc,2}$, energy of beam 2\\
$\delta E_b$, energy spread of each beam\\
$\Delta E_{sep}=E_{acc,2}-E_{stack}$ \\
$\Delta E_{sep,s}$, start of crossing?\\
$\Delta E_{sep,e}$, end of crossing?\\
$\left< \Delta E \right> _D$, energy of phase displacement\\
$f_{stack}$, revolution frequency at $E_{stack}$\\
$h$, harmonic number\\
$n$, integer number\\
$N(t)$, the number of protons circulating \\
$N_s$, the number of stacking \\
$p_\textrm{ref}$, momentum at reference momentum\\
$p_0$, nominal momentum\\
$\delta p/p_0$, relative momentum spread\\
$\Delta p$, deviation of momentum from its nominal value\\
$Q_y$, vertical tune\\
$Q_I$, the nearest integer of $\frac{\omega_{h\beta}}{\omega_{rev}}$  \\
$\Delta Q_y$, space charge tune shift in the vertical direction \\
$R$, average machine radius\\
$t$, time \\
$t_{acc,2}$, acceleration time of beam 2\\
$t_{coast}$, coasting time\\
$T_{user}$, cycle time for users \\
$T_{acc}$, cycle time of accelerator \\
$T$, two times separated by $T$\\
$\beta$, relativistic velocity\\
$\gamma$, Lorentz gamma\\
$\gamma_t$, transition gamma\\
$\varepsilon_{L}$, longitudinal emittance\\
$\varepsilon_{x,y}$, transverse geometrical emittance\\
$\tilde{\beta}_{x,y}$, average $\beta$ function\\
$\eta$, slippage factor \\
$\tau$, lifetime\\
$\phi_s$, synchronous phase\\
$\phi_i$, phase of individual particle\\
$\phi_s$, synchronous phase\\
$\Delta \phi$, horizontal phase advance between RF cavities \\
$\omega_i$, angular frequency of individual particle\\
$\omega_\textrm{ref}$, angular frequency at reference momentum\\
$\omega$, angular frequency\\
$\omega_0$, nominal angular frequency\\
$\omega_\textrm{RF}$, RF angular frequency\\
$\omega_\textrm{rev}$, revolution frequency\\
$\omega_{hb}$, horizontal betatron oscillation frequency\\
$\Delta \omega = \omega_{RF}-h\omega_{rev}$\\
$\delta \omega/\omega_0$, relative frequency spread\\
}
